# Supplementary material for: Runtime Enforcement of CPS against Signal Temporal Logic
Source: arXiv:2502.11584 source file (2025-02-17)
Supplement: Supplementary file 1 [file sec_appendix.tex]

\section*{Appendix}
\label{sec:appendix}
We here provide the proofs of the Propositions.

\subsection{Proof of Proposition \ref{propo1}}
It states that, if a timed word $\sigma$ is accepted by the transducer of Until operator $\automaton_{p_1\until_{[a,b]}p_2}$ then the corresponding signals $\signal$ satisfy $ p\until_{[a,b]}p_2$, i.e.,
        \begin{align*}
            \sigma \in \mathcal{L}(\automaton_{p_1\until_{[a,b]}p_2}) \implies \signal \models p_1\until_{[a,b]}p_2
        \end{align*}

    Proof: Let us consider the following cases based on the events received in time intervals: $[0, a], (a,b]$.
    \begin{enumerate}
        \item Case 1: when the time interval is $[0,a]$:\\
        Based on the events received at $t\in [0,a]$, we have the following sub-cases:
        \begin{enumerate}
            \item Case 1a: $p_1$ is continuously received by the transducer at $t \in [0,a]$ and $p_2$ is received at $t\in[a,a]$.

            The sequence of locations visited by the transducer for this case will be $l_0, l_1, l_2$. Thus, we see that the final location $l_2$ is reached by the transducer, thus $\sigma \in \mathcal{L}(\automaton_{p_1\until_{[a,b]}p_2})$.

            According to the semantics of STL, if $p_2$ is received at $t\in[a, a]$ until that $p_1$ is continuously received, then the STL formula is satisfied by the signals corresponding to $\sigma$. Thus the proposition holds.
            
            \item Case 1b: $p_1$ is not true at $t \in [0,a]$ and $p_2$ is true at $t\in[a,a]$.

            The sequence of locations visited by the transducer for this case will be $l_0, l_1, l_2$. On the way, the transducer modifies the signals $\signal$ to $\signal'$  such that $\signal$ is minimally modified to $\signal'$ (i.e., $min(|\signal'-\signal|))$ and  proposition $p_1$ evaluates to true for $\signal'$ (i.e., $p_1(\signal')=true$). The final location $l_2$ is reached by the transducer, thus $\sigma \in \mathcal{L}(\automaton_{p_1\until_{[a,b]}p_2})$.

            Since after modifying signals by the transducer, $p_1$ is true until $p_2$ is received at $t\in[a, a]$, thus according to the semantics of STL, the STL formula is satisfied and the proposition holds.\\
            
        \end{enumerate}
        \item Case 2: when the time interval is $(a,b]$:\\
         Based on the events received at $t\in (a,b]$, we have the following sub-cases:
        \begin{enumerate}
            \item Case 2a: $p_2$ is received by the transducer at $t \in (a,b]$ and $p_1$ is continuously received until that.
            
            The sequence of locations visited by the transducer for this case will be $l_0, l_1, l_3, l_2$. Thus, we see that the final location $l_2$ is reached by the transducer, thus $\sigma \in \mathcal{L}(\automaton_{p_1\until_{[a,b]}p_2})$.

            According to the semantics of STL, if $p_2$ is received at $t\in (a,b]$ until that $p_1$ is continuously received, then the STL formula is satisfied by the signals corresponding to $\sigma$. Thus the proposition holds.

            \item Case 2b: $p_1$ is true at $t \in 
            (a,b]$ and $p_2$ is not true at $t\in(a,b]$.

            The sequence of locations visited by the transducer for this case will be $l_0, l_1, l_2, l_3$. The transducer modifies the signals $\signal$ to $\signal'$  at $t \in [b,b]$ such that $\signal$ is minimally modified to $\signal'$ (i.e., $min(|\signal'-\signal|))$ and  proposition $p_2$ evaluates to true for $\signal'$ (i.e., $p_2(\signal')=true$). The final location $l_2$ is reached by the transducer, thus $\sigma \in \mathcal{L}(\automaton_{p_1\until_{[a,b]}p_2})$.

            Since after modifying signals by the transducer, $p_2$ is true at $t \in [b,b]$ and until that $p_1$ is true at $t\in (a,b]$, thus according to the semantics of STL, the STL formula is satisfied and the proposition holds.

             Case 2c: $p_1$ and $p_2$ is not true at $t\in(a,b]$.

             The sequence of locations visited by the transducer for this case will be $l_0, l_1, l_2, l_3$. On the way, the transducer modifies the signals $\signal$ to $\signal'$  at $t \in (a,b])$ such that $\signal$ is minimally modified to $\signal'$ (i.e., $min(|\signal'-\signal|))$ and  proposition $p_1$ evaluates to true for $\signal'$ (i.e., $p_1(\signal')=true$). Also, the transducer modifies the signals $\signal$ to $\signal'$  at $t \in [b,b]$ such that $\signal$ is minimally modified to $\signal'$ (i.e., $min(|\signal'-\signal|))$ and  proposition $p_2$ evaluates to true for $\signal'$ (i.e., $p_2(\signal')=true$).              
             The final location $l_2$ is reached by the transducer, thus $\sigma \in \mathcal{L}(\automaton_{p_1\until_{[a,b]}p_2})$.

             Since after modifying signals by the transducer, $p_2$ is true at $t \in [b,b]$ and until that $p_1$ is true at $t\in (a,b]$, thus according to the semantics of STL, the STL formula is satisfied and the proposition holds.
        \end{enumerate}
    \end{enumerate}
A similar proof can be given for the Release operator of STL and its transducer.
%%%%%%%%%%%%%%%%%%%%%%%%%%%%%%%

\subsection{Proof of Proposition \ref{propo3}}
It states that, if signals  satisfy the Until formula $ \varphi_1\until_{[a,b]}\varphi_2$, then its encoded word is accepted by its transducer, i.e., 
    \begin{align*}
        \signal \models \varphi_1\until_{[a,b]}\varphi_2 \implies \sigma \in 
        \mathcal{L}(\automaton_{\varphi_1\until_{[a,b]}\varphi_2}) 
    \end{align*}

    Proof: Let us consider the following cases based on the events received in time intervals: $[0, a], (a,b]$.
    \begin{enumerate}
        \item Case 1: when the time interval is $[0,a]$: an STL formula is satisfied at $t\in [0, a]$ by signals $\signal$, if $p_1$ of the encoded word $\sigma$ of $\signal$ is continuously true and $p_2$ of the encoded word $\sigma$ of $\signal$ is true at $t\in[a, a]$.

        For the encoded word $\sigma$ of signals $\signal$, the transducer makes a sequence of transitions involving locations $l_0, l_1, l_2$ and goes to the accepting state $l_2$. Thus,  $\sigma \in 
        \mathcal{L}(\automaton_{\varphi_1\until_{[a,b]}\varphi_2})$. and proposition holds.

        \item  Case 2: when the time interval is $(a,b]$: an STL formula is satisfied at $t\in (a,b]$ by signals $\signal$, if $p_2$ of the encoded word $\sigma$ of $\signal$ is received at $t\in (a,b]$ and  $p_1$ of the encoded word  $\sigma$ of $\signal$  is continuously true until that.

        For the encoded word $\sigma$ of signals $\signal$, the transducer makes a sequence of transitions involving locations $l_0, l_1, l_3, l_2$ and goes to the accepting state $l_2$. Thus,  $\sigma \in 
        \mathcal{L}(\automaton_{\varphi_1\until_{[a,b]}\varphi_2})$. and proposition holds.
    \end{enumerate}

A similar proof can be given for the Release operator of STL and its transducer.
